# Supplementary material for: Simple crowd dynamics to generate complex temporal contact networks
Source: arXiv:2405.06508 ancillary file (2025-03-19)
Supplement: Supplementary file 1 [file appendix.pdf]

# Simple crowd dynamics to generate complex temporal contact networks

## Supplementary information

Razieh Masoumi<sup>1,2</sup>, Juliette Gambaudo<sup>1</sup>, and Mathieu G  nois<sup>1</sup>

<sup>1</sup> Aix-Marseille Universit  , CNRS, CPT, Marseille, France and

<sup>2</sup> Department of Molecular Medicine, Universit   of Padova, Italy.

(Dated: December 9, 2024)

### MODELS

### Vicsek model

#### Description

##### Random walk

In the 2D Random Walk, each walker selects a random direction at each subsequent step, uniformly distributed between 0 and  $2\pi$ , with a step length of  $\Delta r$ . The value of  $\Delta r$  is drawn at random in the positive half of a Gaussian distribution of mean 0 and of variance  $D*dt$ , where  $D$  and  $dt$  represent the diffusion coefficient and time increment at each step respectively. This continuous randomness in the particle's movements is classically known to be a good model for a brownian motion [1]. The diffusion coefficient allows us to control the characteristics of the random walk. For a given time increment  $dt$ , a larger diffusion coefficient implies that the random walker is more likely to move and spread rapidly throughout its surrounding space.

The Vicsek model focuses on collective behavior emerging from local interactions among self-propelled particles. Inspired by the movement of flocks of birds or schools of fish, this model assumes that particles align their velocities with those of their neighbors within a certain interaction radius  $R_n$ , while accounting for uncertainties caused by noise  $\eta_i$ . This alignment is mathematically described by the following equation:

$$\Theta_i(t + \Delta t) = \langle \Theta_j \rangle_{|\mathbf{r}_i - \mathbf{r}_j| < R_n} + \eta_i,$$

where  $\Theta_i(t)$  indicates the angle defining the direction of the velocity of particle  $i$ , while  $\langle \Theta_j \rangle_{|\mathbf{r}_i - \mathbf{r}_j| < R_n}$  signifies the average angle of velocity vectors among the neighboring particles of particle  $i$  within a distance of  $R_n$ . Hence, the particle moves at constant speed  $v$  in new direction according to the following equation:

$$\mathbf{r}_i(t + \Delta t) = \mathbf{r}_i(t) + \mathbf{v}\Delta t \begin{pmatrix} \cos \Theta_i(t) \\ \sin \Theta_i(t) \end{pmatrix},$$

where  $\mathbf{r}_i(t)$  indicates the position of particle  $i$  at time  $t$ .

##### Active Brownian Particles (ABP)

The Active Brownian Particle (ABP) model adds a layer of complexity by adding a memory aspect into the particle motion. In the classical version of this model, particles undergo both a Brownian motion and a deliberate movement (usually the consequence of internal energy sources or external driving forces). In our simplified version, we exclude Brownian motion affecting position and focus solely on the self-propulsion of particles [2].

In practice, particles are constrained at each time step to select a new orientation uniformly within a specific range of angles, namely  $\Delta\theta = [-\frac{\theta}{2}, \frac{\theta}{2}]$  around their current orientation, while maintaining a constant velocity  $v$ .

In this model, trajectories of particles exhibit a persistence of the angle over the persistence length, which increases as the angle range  $\Delta\theta$  decreases. Note that for  $\Delta\theta = 2\pi$ , the ABP model is simply the 2D Random Walk with fixed step length.

### Computing contacts

An interaction between particles is defined by two factors: the closeness of particles to each other and the orientation with which particles can detect each other. As illustrated in Fig. 2, particles can only detect another particle present in their front half circle, which is characterized by a detection radius  $r_D$  and a detection vector named  $\vec{D}_i$  for particle with index  $i$ . For the sake of simplicity, we assume that the detection vector for each particle coincides with the velocity vector of the particle. This assumption is logically sound, as in most contact cases the orientation of the line of sight coincides with the movement. We further assume a similar detection radius of  $r_D = 1$  for all particles.

Let us consider two particles  $A$  and  $B$  separated by a distance less than  $r_D$ . Let  $\vec{AB}$  be the vector from particle  $A$  to particle  $B$ . Particle  $B$  is then within the detection area of Particle  $A$  if  $\vec{AB} \cdot \vec{D}_A \geq 0$ . Similarly, Particle  $A$  is within the detection area of Particle  $B$  if  $\vec{AB} \cdot \vec{D}_B \leq 0$ . The fulfillment of both these conditions is necessary to establish that the two particles are in contact.

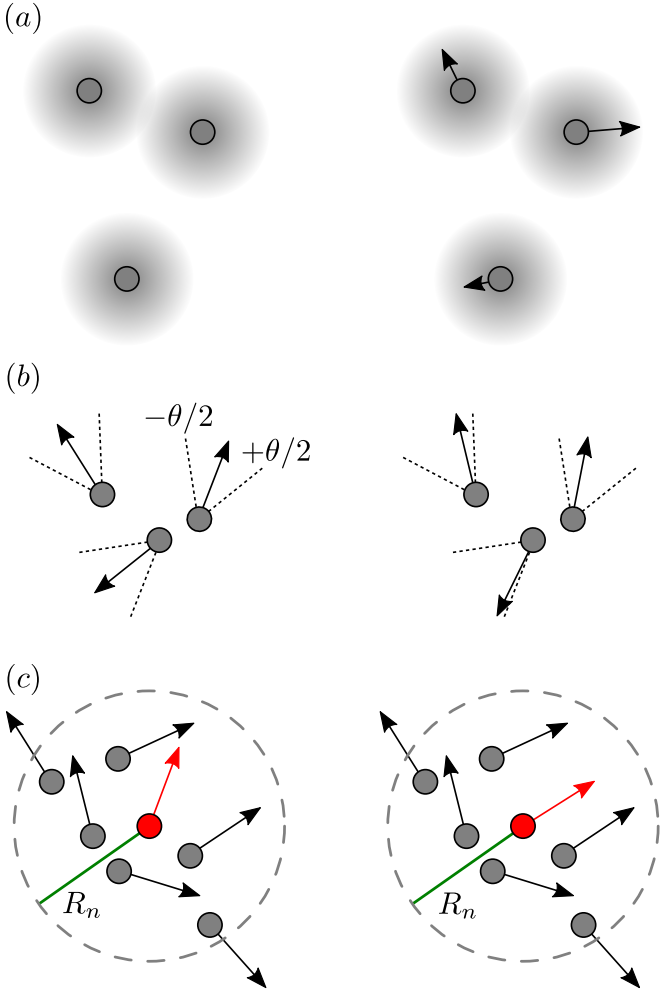

FIG. 1. **Schematic representation of the motion mechanisms for the three models.** (a) 2D Random Walk: at each time step, each particle selects a direction and a step length at random, following a uniform distribution for the angle and a half-gaussian for the step length. (b) Active Brownian Particle: at each time step, each particle updates its direction  $\alpha$  by selecting uniformly at random a variation  $\Delta\alpha$ , with  $\Delta\alpha$  constrained within the range  $[-\frac{\theta}{2}, \frac{\theta}{2}]$ , while maintaining of a constant velocity  $v$ . The smaller  $\theta$ , the more the particle exhibits persistence of the direction of its motion. (c) Vicsek model: at each time step, particles align their direction with their neighbors by selecting the average direction over all neighbors within a given radius  $R_n$ . The alignment is altered by a noise  $\eta$  similar to the ABP model.

### EFFECT OF PARTICLE SIZE AND BOUNDARY CONDITIONS ON INTER-CONTACT DURATIONS

In order to better understand the possible mechanisms responsible for the peculiar shape of the distribution of inter-contact durations, we focus on the 2D Random Walk and modified the way particles interact as well as the boundary conditions. For the particle size, the main difference between point particles and finite-size parti-

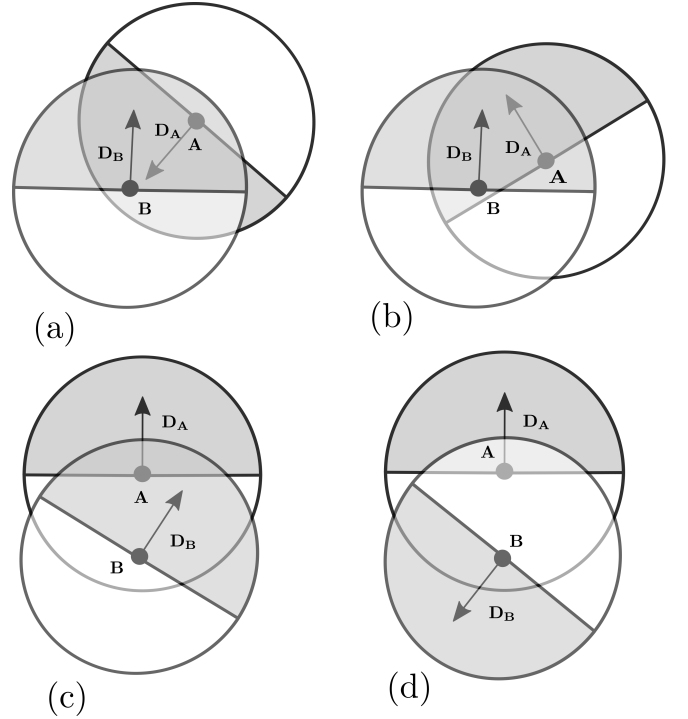

FIG. 2. **Typical four situations for particle contacts.** When two particles A and B are closer than the detection radius  $r_D$ , four different situations can occur depending on their respective orientation vectors  $D_A$  and  $D_B$ . As per our defined concept of contact, particles A and B are deemed to be in contact in configurations (a) and (b), as they are in both cases facing each other, *i.e.* in their respective front half-discs. In configurations (c) and (d) however, they are not in such a configuration and thus not considered to be in contact.

cles is the spatial organization: point particles can be as numerous as possible in a defined area of the simulated space and thus have unlimited simultaneous interactions, while the volume occupied by finite-size particles leads to a spatial organization and limits the number of simultaneous interactions. Changes in boundary conditions can modify the behaviour of a system. Hard boundaries impact the trajectories of particles while periodic boundaries do not; hard boundaries and periodic boundaries may impose finite-size effect on the global dynamics of the system while open boundaries do not.

As seen on Figure 3, changes in the particle size or in the boundary conditions do not affect at all the distribution of inter-contact durations, which retains in all cases its power law tail with an exponent  $-1.5$ . In particular, it works for the case of point particles doing a random walk with no boundaries. This very simple setting allows us to analytically derive the distribution.

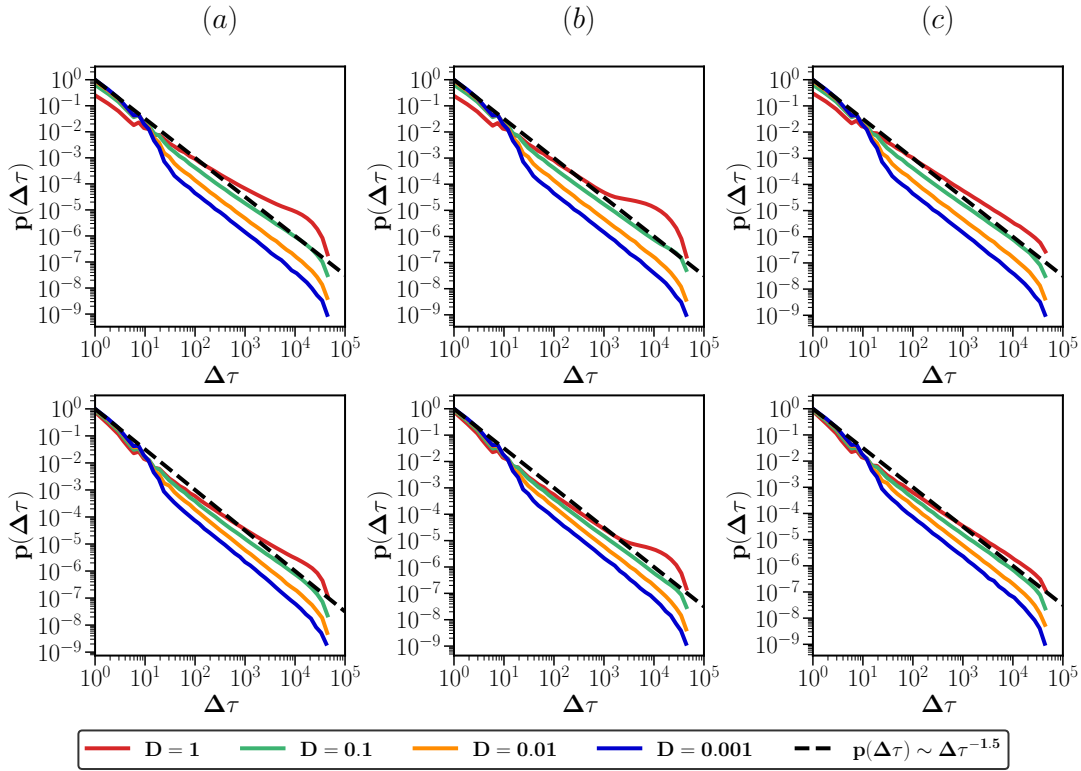

FIG. 3. Comparison of the distributions of inter-contact durations for the different version of the 2D Random Walk. Top: point particles, bottom: finite size particles. (a) Hard boundaries, (b) Periodic boundaries, (c) No boundaries.

### ANALYTICAL ARGUMENT FOR THE DISTRIBUTION OF INTERCONTACT DURATIONS

For the 2D Random Walk of point particles on an infinite space, we first acknowledge that the trajectories of particles are uncorrelated, as they do not interact. The distribution of inter-contact durations for a population of particles is thus strictly identical as the one for only 2 particles.

Then, the system can be reduced to tracking the evolution of the distance  $d$  between the two particles. If we define the random walk with the following process:

$$\mathbf{x}(t+1) = \mathbf{x}(t) + \mathbf{r} \quad (1)$$

with  $\mathbf{r}$  a random vector with an angle  $\theta$  chosen uniformly in  $[0, 2\pi[$  and a norm  $r$  chosen following the positive half of a gaussian, we have then:

$$\mathbf{d}_{12}(t+1) = \mathbf{d}_{12}(t) + \mathbf{s} \quad (2)$$

with  $\mathbf{s} = \mathbf{r}_2 - \mathbf{r}_1$ . Given Eq. (1),  $\mathbf{s}$  is also a random vector, which angle follows a uniform distribution. This indicates that  $\mathbf{d}$  follows a 2D random walk process. As a consequence, the evolution of its norm  $d$  can be written as a 1D random walk process.

The distribution of inter-contact durations is then the distribution of the time it takes for  $d$ , starting from

$d \leq r_D$ , to become smaller than the detection radius  $r_D$  again. This distribution is exactly the distribution of first return times for the associated 1D random walk. Independently from the details of the stochastic process governing the evolution of  $d$ , this distribution has a power law tail  $p(\Delta\tau) \sim \Delta\tau^{-3/2}$  [3], which is precisely the exponent we observe numerically.

- 
- [1] Gregory F Lawler and Vlada Limic. *Random walk: a modern introduction*, volume 123. Cambridge University Press, 2010.
  - [2] Pawel Romanczuk, Markus Bär, Werner Ebeling, Benjamin Lindner, and Lutz Schimansky-Geier. Active brownian particles: From individual to collective stochastic dynamics. *The European Physical Journal Special Topics*, 202:1–162, 2012.
  - [3] Sidney Redner. *A Guide to First-Passage Processes*. Cambridge University Press, 2001.

### ADDITIONAL SIMULATION PLOTS

In this section we present additional plots to provide a complete overview of the models' behaviour.

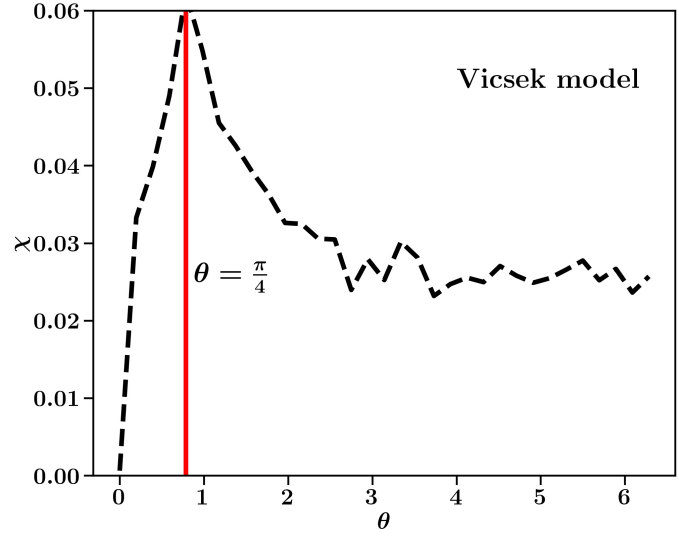

FIG. 4. **Phase transition of the Vicsek model.** We compute the variance of the local average velocity as a function of the noise angle  $\theta$ . This variance exhibits a maximum for  $\theta \simeq \frac{\pi}{4}$ , indicating where the transition between the random phase and the flocking phase occurs for the density of particles we set.

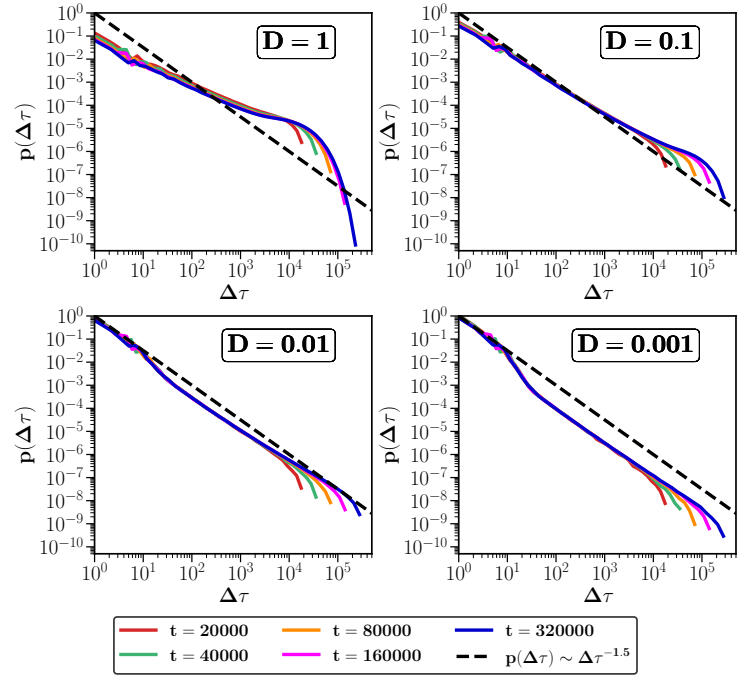

FIG. 5. **Stability of the distribution of intercontact duration with time – 2D random walk.** Model with point particles and hard boundaries.

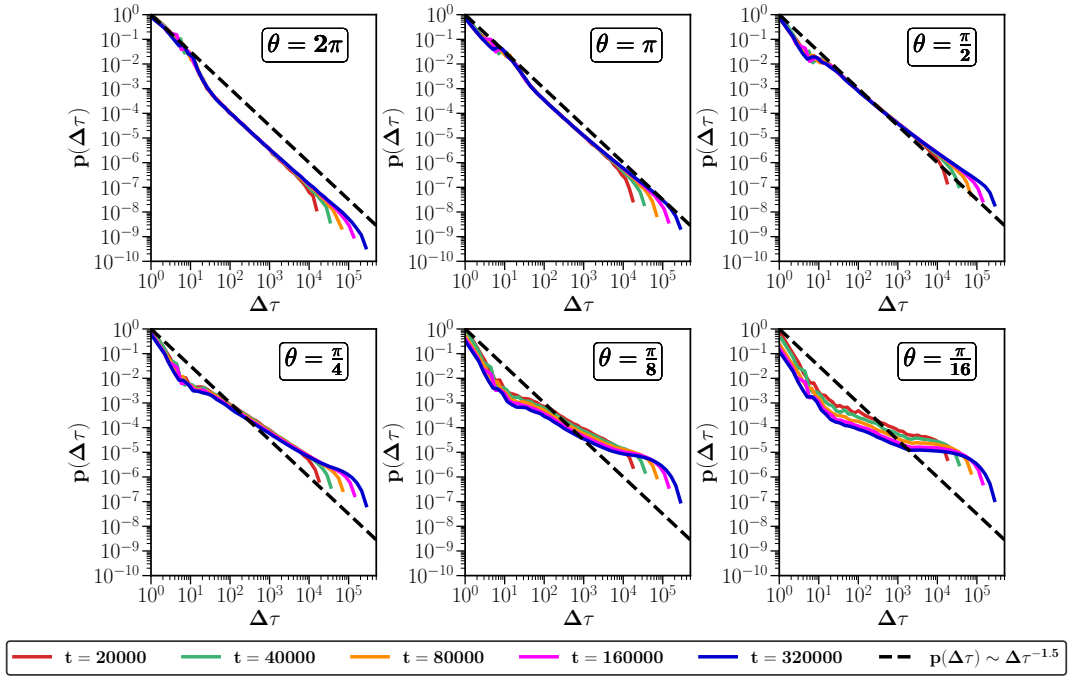

FIG. 6. **Stability of the distribution of intercontact duration with time – ABP.** Model with point particles and hard boundaries.

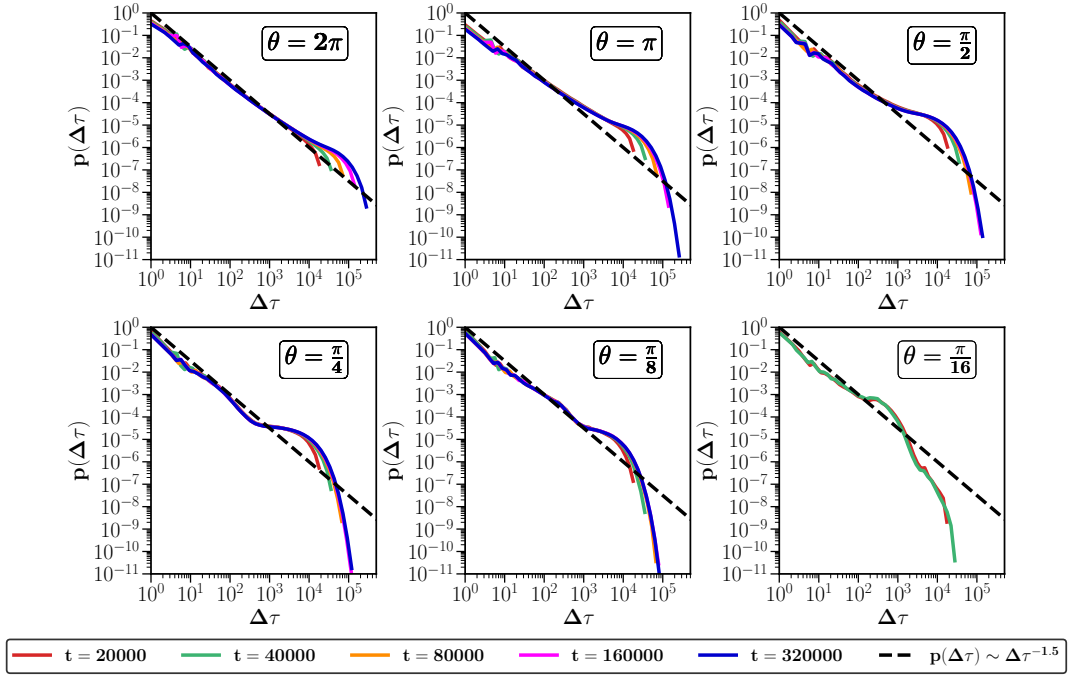

FIG. 7. **Stability of the distribution of intercontact duration with time – Vicsek.** Model with point particles and hard boundaries.

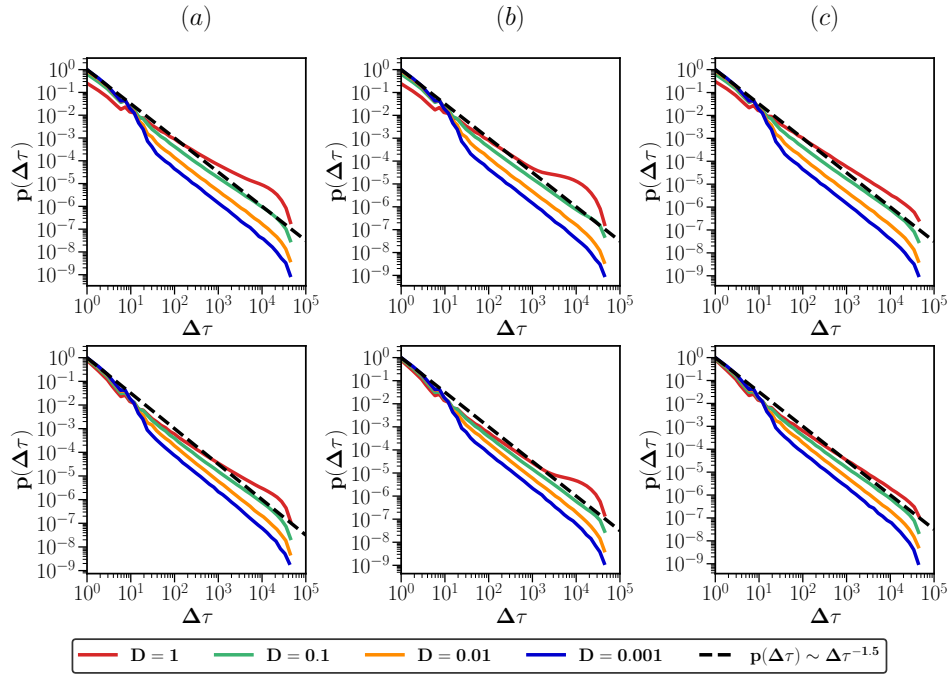

FIG. 8. Comparison of the distributions of inter-contact durations for the different version of the 2D random walk. Top: point particles, bottom: finite size particles. (a) Hard boundaries, (b) Periodic boundaries, (c) No boundaries.

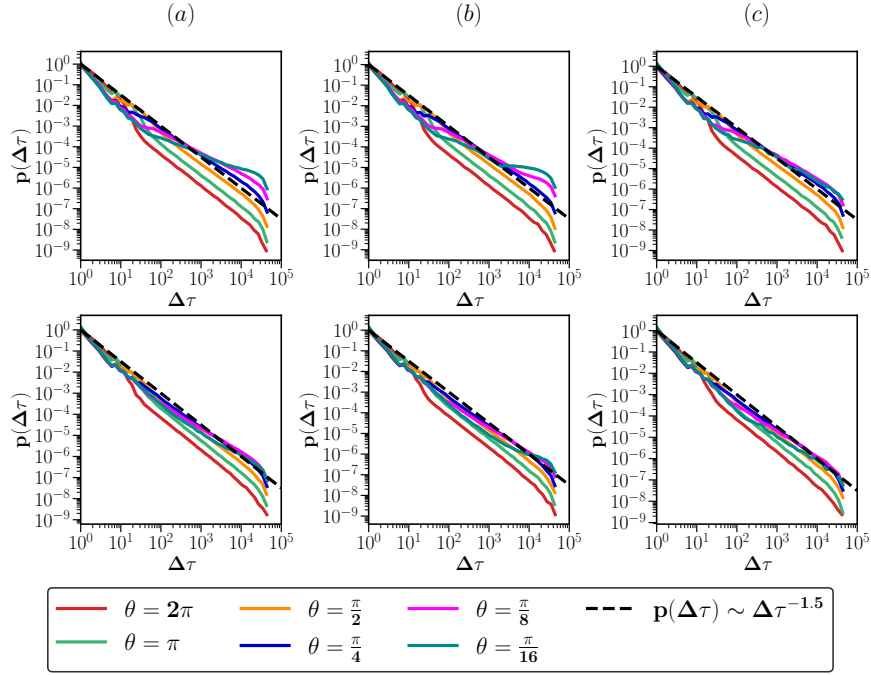

FIG. 9. Comparison of the distributions of inter-contact durations for the different version of the ABP. Top: point particles, bottom: finite size particles. (a) Hard boundaries, (b) Periodic boundaries, (c) No boundaries.

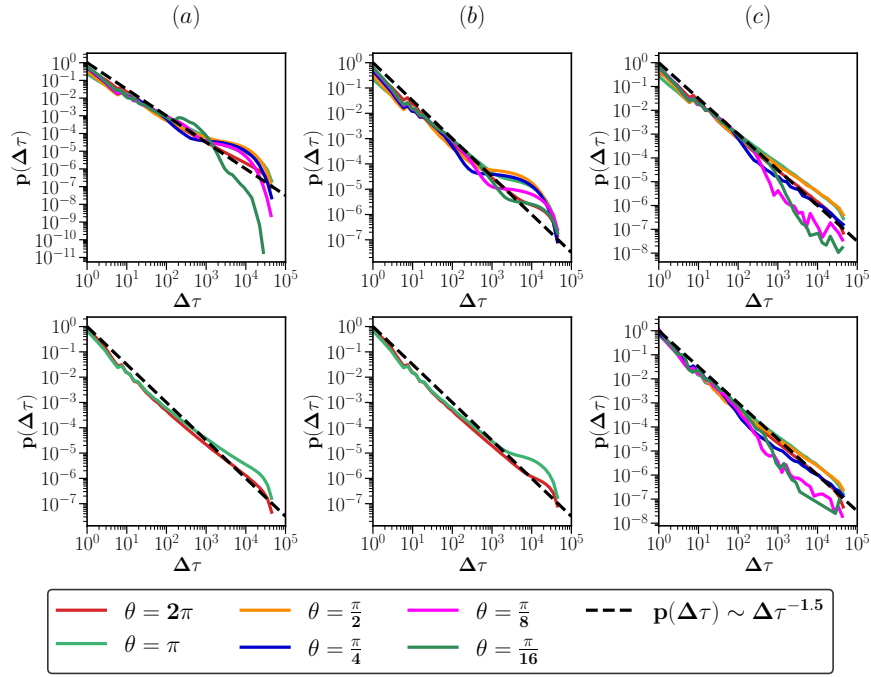

FIG. 10. **Comparison of the distributions of inter-contact durations for the different version of the Vicsek model.** Top: point particles, bottom: finite size particles. (a) Hard boundaries, (b) Periodic boundaries, (c) No boundaries. Simulations are missing in two plots, due to the difficulty of simulating the system with many interactions for particles with size.

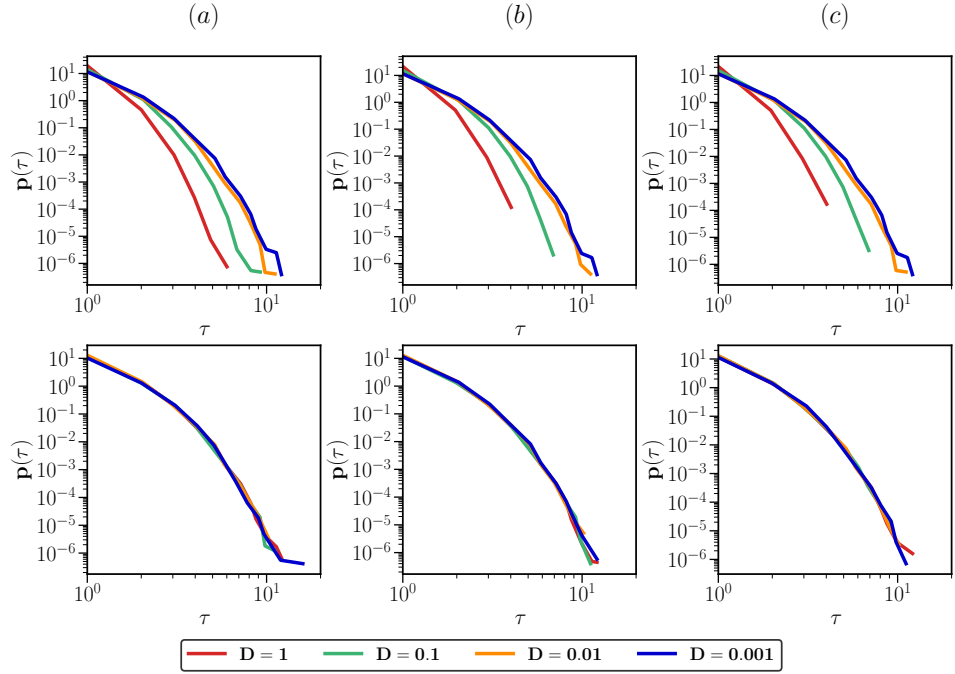

FIG. 11. **Comparison of the distributions of contact durations for the different version of the 2D random walk.** Top: point particles, bottom: finite size particles. (a) Hard boundaries, (b) Periodic boundaries, (c) No boundaries.

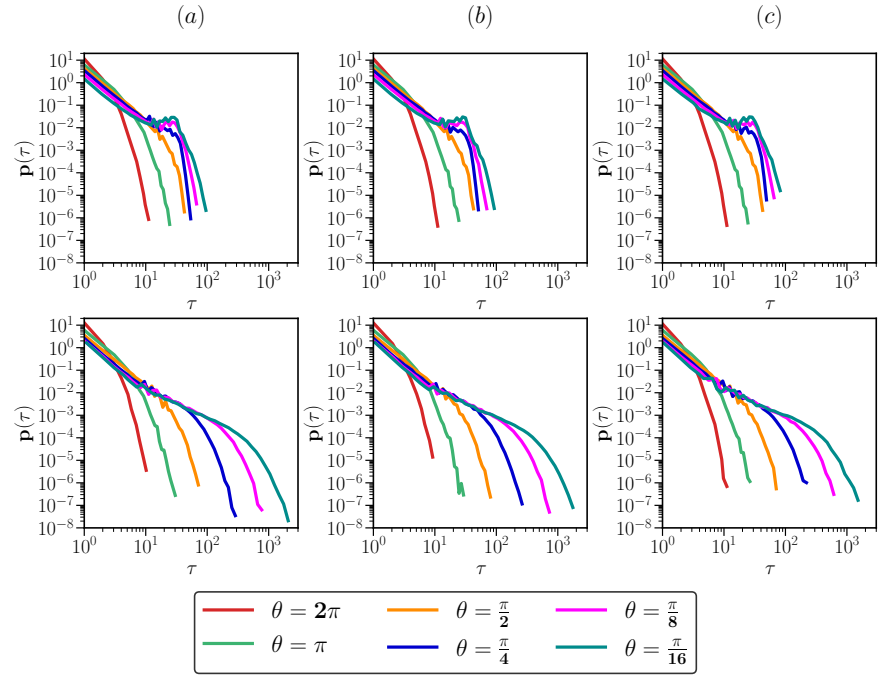

FIG. 12. Comparison of the distributions of contact durations for the different version of the ABP model. Top: point particles, bottom: finite size particles. (a) Hard boundaries, (b) Periodic boundaries, (c) No boundaries.

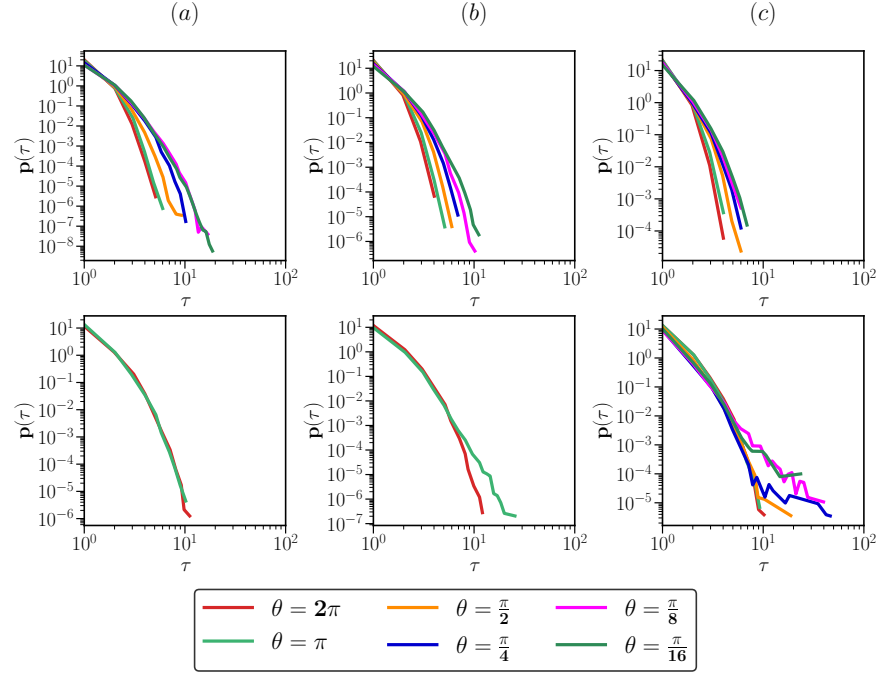

FIG. 13. Comparison of the distributions of contact durations for the different version of the Vicsek model. Top: point particles, bottom: finite size particles. (a) Hard boundaries, (b) Periodic boundaries, (c) No boundaries. Simulations are missing in two plots, due to the difficulty of simulating the system with many interactions for particles with size.

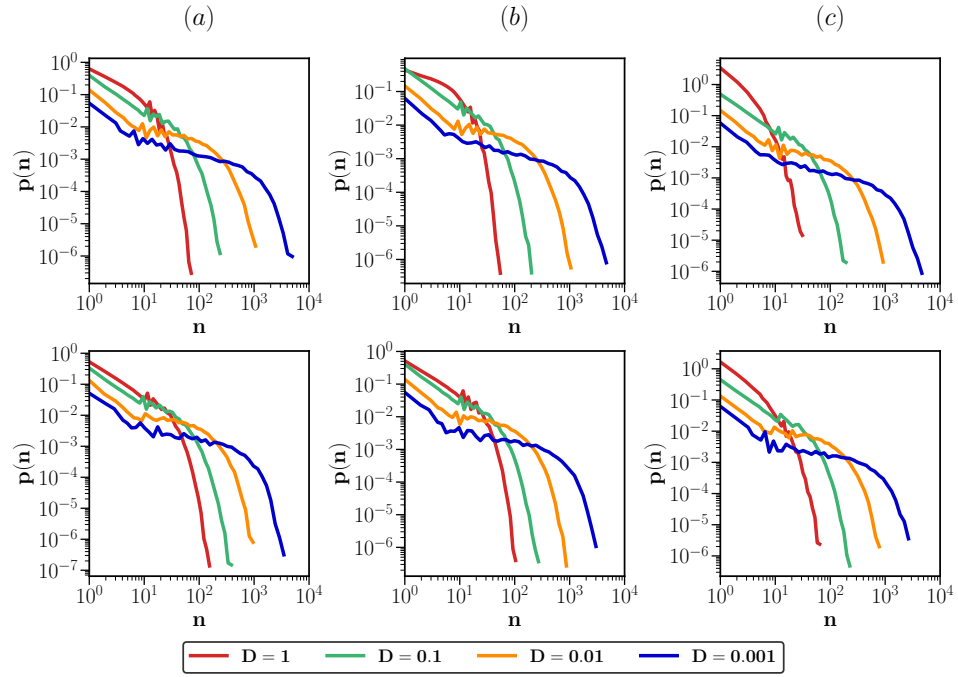

FIG. 14. **Comparison of the distributions of number of contacts for the different version of the 2D random walk.** Top: point particles, bottom: finite size particles. (a) Hard boundaries, (b) Periodic boundaries, (c) No boundaries.

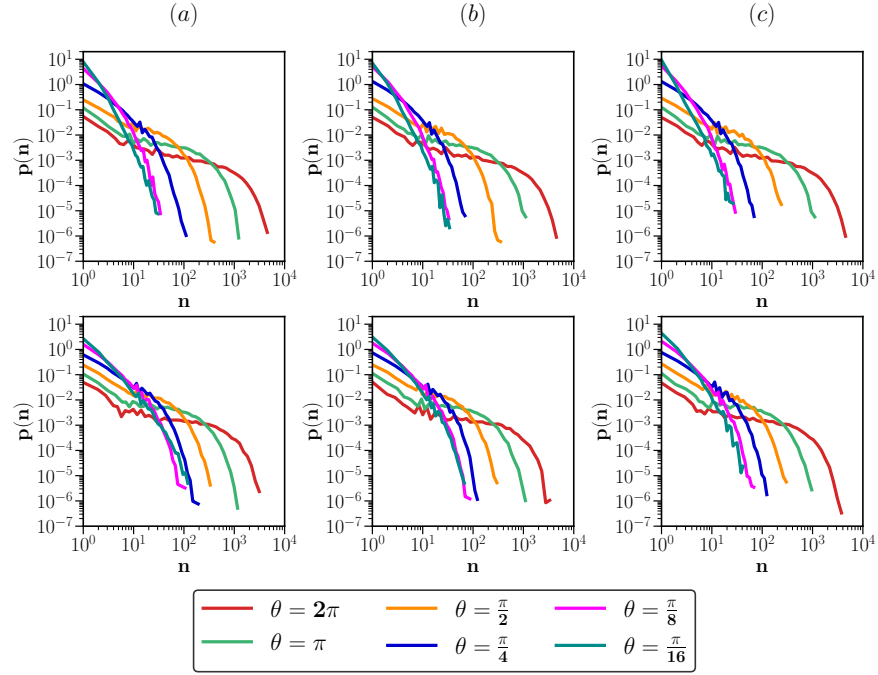

FIG. 15. **Comparison of the distributions of number of contacts for the different version of the ABP model.** Top: point particles, bottom: finite size particles. (a) Hard boundaries, (b) Periodic boundaries, (c) No boundaries.

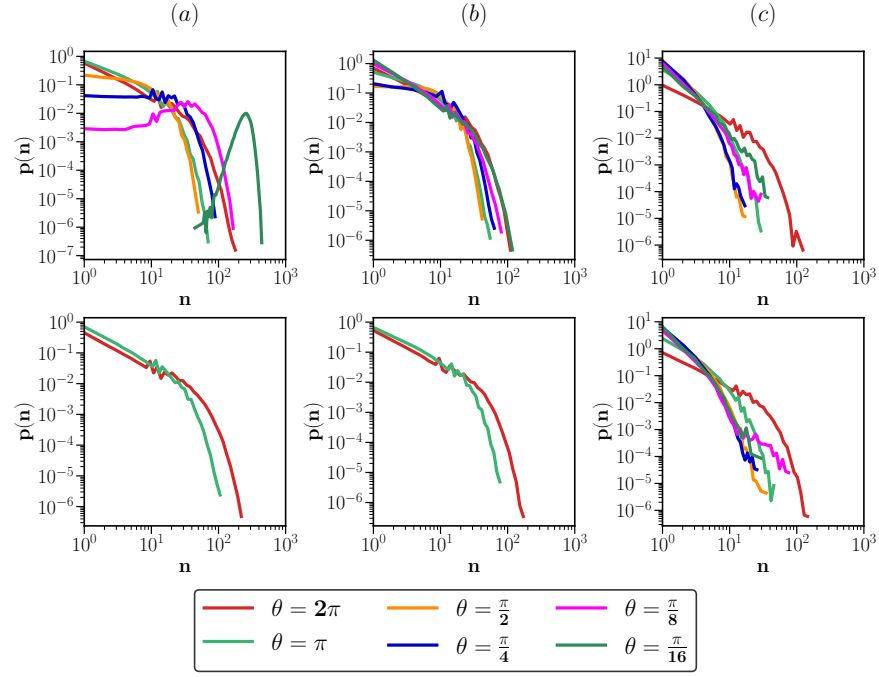

FIG. 16. **Comparison of the distributions of number of contacts for the different version of the Vicsek model.** Top: point particles, bottom: finite size particles. (a) Hard boundaries, (b) Periodic boundaries, (c) No boundaries. Simulations are missing in two plots, due to the difficulty of simulating the system with many interactions for particles with size.

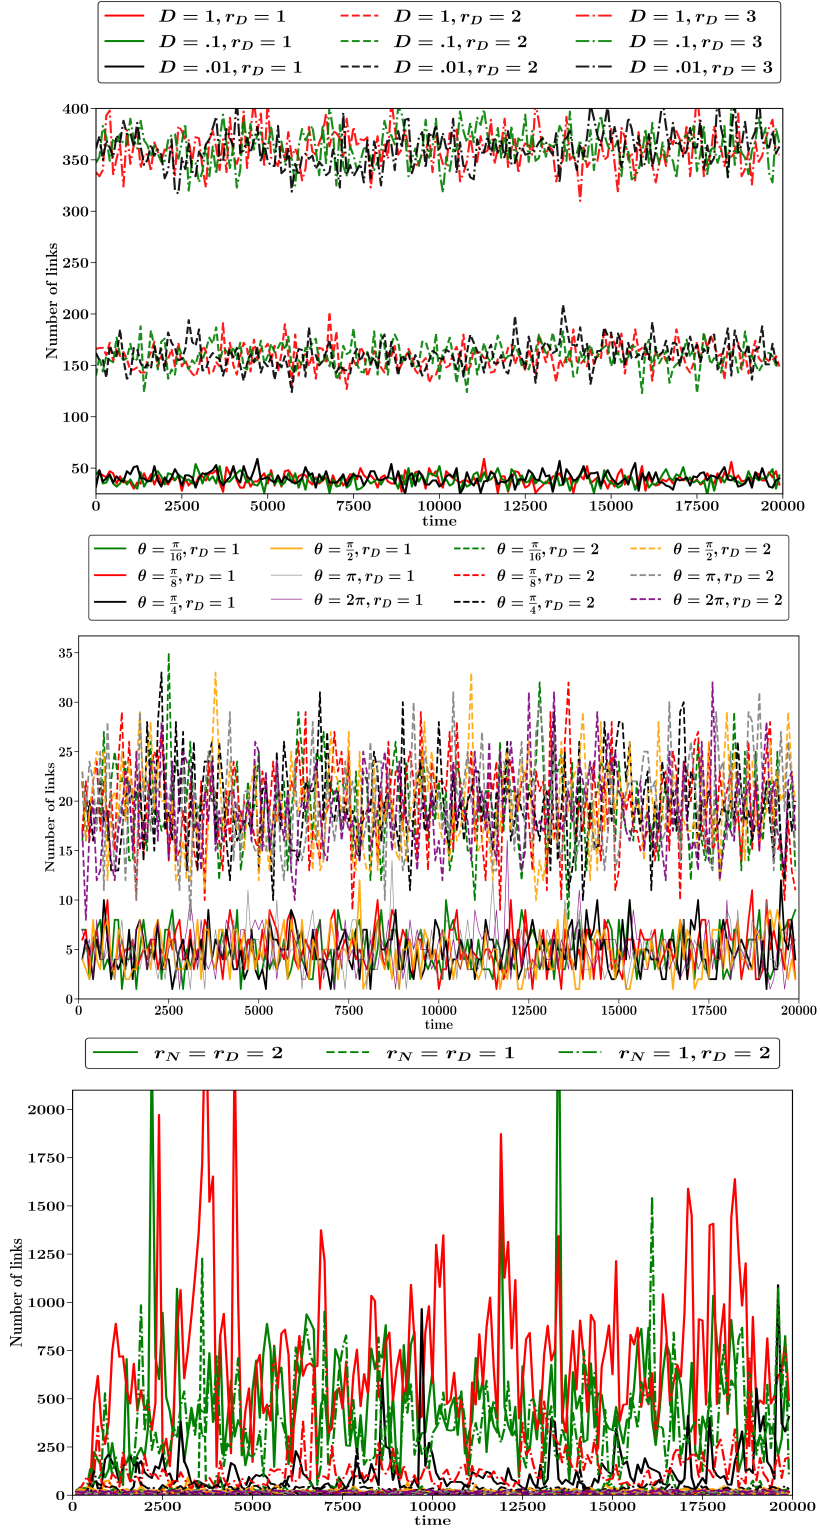

FIG. 17. **Number of contacts as a function of time.** Top: 2D random walk; middle: ABP; bottom: Vicsek model. Both 2DRW and ABP exhibit a stationarity of the number of contacts in time. For the Vicsek model, the random phase also exhibit such a stationarity (as it is roughly equivalent to the previous two) while in the flocking phase the number of contacts exhibits large deviations due to the numerous interactions occurring within the flocks.

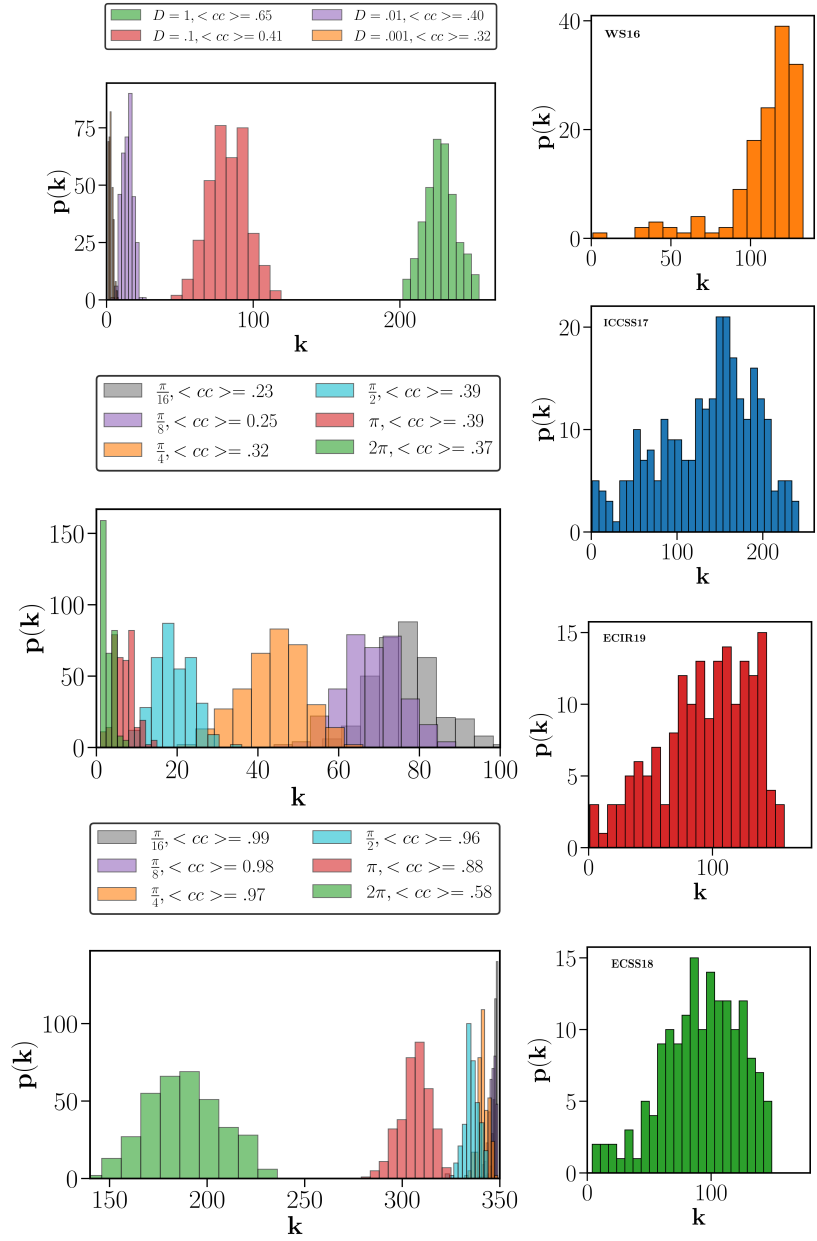

FIG. 18. **Aggregated degree distributions.** We compute the degree distributions of for the temporal networks aggregated along time, for a simulation time of  $t = 50000$  time steps and 350 particles. Top: 2D random walk; middle: ABP; bottom: Vicsek model; right column: empirical data. For 2DRW, as the diffusion coefficient increases, the mean degree of the network shifts towards higher values. For ABP, a narrower range of angles results in increasing the mean degree. For Vicsek, a decrease in noise levels is associated with a shift towards larger mean degrees as the system enters the flocking phase.
